# Supplementary material for: Allometric scaling of brain activity explained by avalanche criticality
Source: arXiv:2512.10834 source file (2025-12-11)
Supplement: Supplementary file 1 [file SI.pdf]

# SUPPLEMENTARY INFORMATION
# Allometric scaling of brain activity explained by avalanche criticality

Tiago S. A. N. Simões,[1] José S. Andrade Jr.,[2] Hans J. Herrmann,[2,3] Stefano Zapperi,[4,5] and Lucilla de Arcangelis[1]

[1] *University of Campania "Luigi Vanvitelli", Department of Mathematics and Physics, Caserta, Viale Lincoln, 5, 81100, Italy*

[2] *Universidade Federal do Ceará, Departamento de Física, Fortaleza, Ceará, 60451-970, Brazil*

[3] *ESPCI, PMMH, Paris, 7 quai St. Bernard, 75005, France*

[4] *Center for Complexity and Biosystems, Department of Physics, University of Milan, via Celoria 16, 20133 Milano, Italy*

[5] *CNR - Consiglio Nazionale delle Ricerche, Istituto di Chimica della Materia Condensata e di Tecnologie per l'Energia, Via R. Cozzi 53, 20125 Milano, Italy*

## S1. AVALANCHE SIZE AND DURATION DISTRIBUTIONS

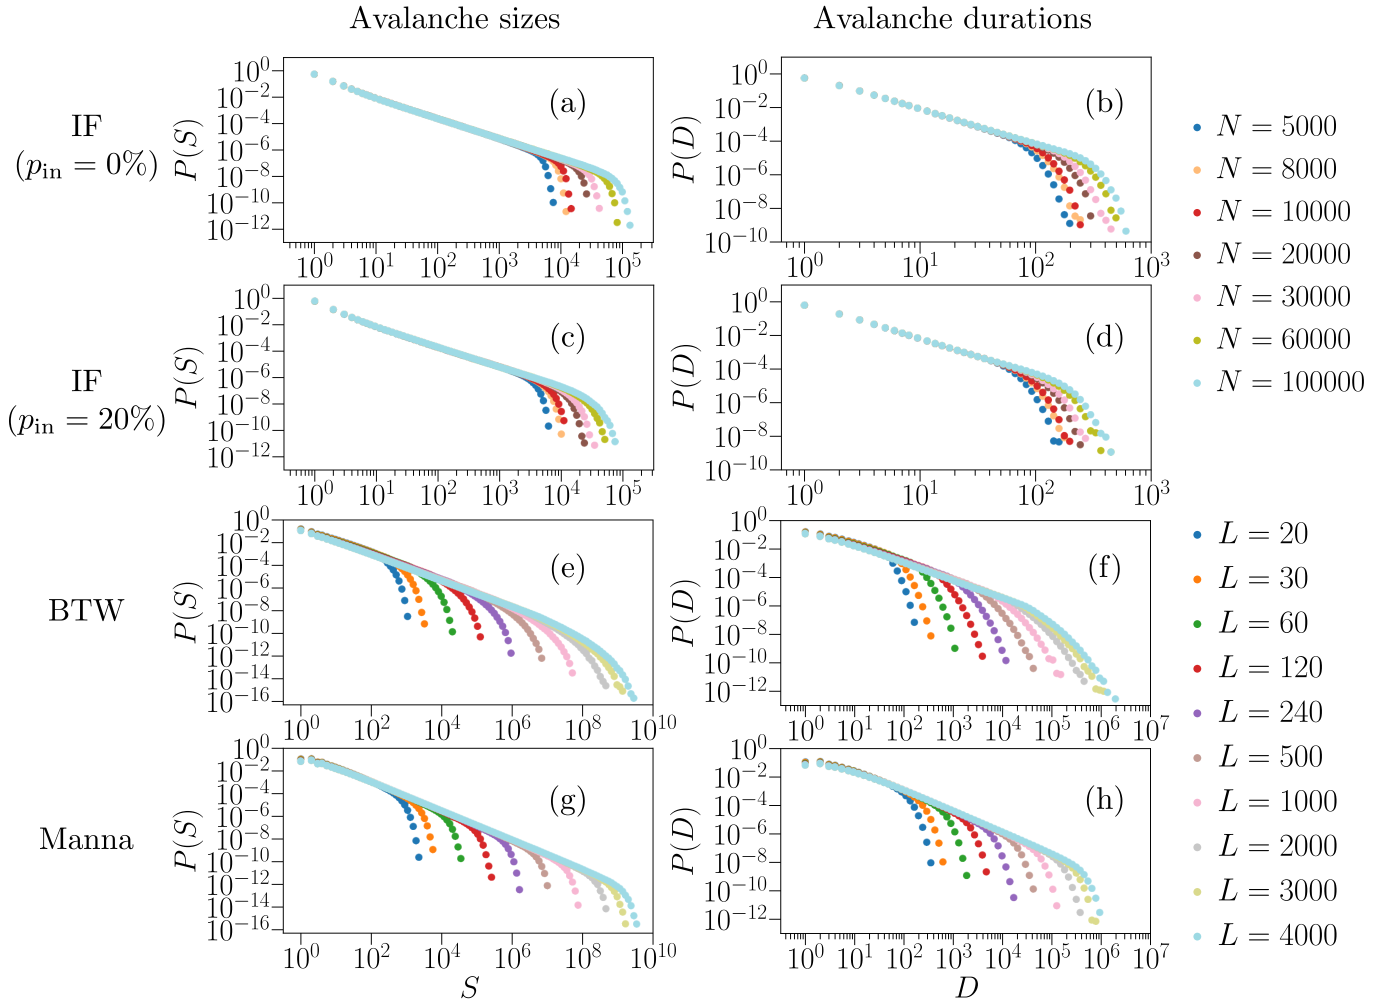


FIG. S1. **Avalanche size and duration distributions.** Distributions of avalanche size $P(S)$ (first column) and duration $P(D)$ (second column) for the IF model with $p_{\rm in} = 0\%$ inhibitory neurons (a-b) and $p_{\rm in} = 20\%$ (c-d), for system sizes $N \in [5000, 100000]$ and for the BTW (e-f) and Manna (g-h) sandpile models, for linear system sizes $L = \sqrt{N} \in [20, 4000]$. The values of $\delta u_{\rm rec}$ that tune the IF networks to the critical state for each $N$ and $p_{\rm in}$ are reported in Table (S1).

TABLE S1. Values of the tuning parameter $\delta u_{\rm rec}$ of the IF model used to obtain the results presented in Fig. (S1)a-d

| **System size** $N$ | $\delta u_{\bf rec}$ ($p_{\bf in} = 0\%$) | $\delta u_{\bf rec}$ ($p_{\bf in} = 20\%$) |
|---|---|---|
| 5000 | $7.50 \cdot 10^{-5}$ | $1.00 \cdot 10^{-4}$ |
| 8000 | $6.00 \cdot 10^{-5}$ | $7.80 \cdot 10^{-5}$ |
| 10000 | $5.30 \cdot 10^{-5}$ | $6.70 \cdot 10^{-5}$ |
| 20000 | $3.80 \cdot 10^{-5}$ | $4.60 \cdot 10^{-5}$ |
| 30000 | $3.10 \cdot 10^{-5}$ | $3.50 \cdot 10^{-5}$ |
| 60000 | $2.20 \cdot 10^{-5}$ | $2.40 \cdot 10^{-5}$ |
| 100000 | $1.70 \cdot 10^{-5}$ | $1.80 \cdot 10^{-5}$ |

## S2. SCALING OF THE AVERAGE $\langle X\rangle$ WITH $N$

In the critical state, according to the finite size-scaling assumption [1], quantities such as $S$ and $D$ follow a power-law distribution with a cut-off in finite systems,

$$P(X) = A_X f(X) X^{-\alpha_X} g(X/X_c), \text{ for } X \in [1, \infty[ \tag{S1}$$

where $X \in \{S, D\}$ represents either the avalanche size $S$ or duration $D$, $A_X$ is the normalization constant, determined by $\int_1^\infty P(X)dX = 1$, where we approximated the sum $\sum_{X=1}^{\infty}$ to an integral. Moreover, $f(X)$ is a correction factor which accounts for possible deviations from the power-law for small $X$, with $f(X) \approx 1$ when $X \gg 1$, $\alpha_X > 0$, and $g(X/X_c)$ is a scaling function that models the cut-off, where $X_c \propto N^{\beta_X}$, with $\beta_X > 0$, defines the value of $X$ for which $g(X/X_c)$ starts to dominate. Furthermore, $g(X/X_c) \approx 1$ for $X < X_c$ while, for $X > X_c$, it decreases rapidly enough to zero, to ensure that at least the first-order moment $\langle X\rangle = \int_1^\infty XP(X)dX \propto \int X^{1-\alpha_X} g(X/X_c)dX$ is finite for finite $N$.

Our intention in this section is to calculate the $\lim_{N\to\infty}\langle X\rangle$. To start, we can estimate the behaviour of $\lim_{N\to\infty} A_X$.

### S2.1. Large $N$ limit of $A_X$

Let $X_f$ be such that $f(X) = 1$ if $X > X_f$. Then, using the normalization condition and separating the integral into three parts,

$$1 = \int_1^\infty P(X)dX = A_X \cdot \left( \overbrace{\int_1^{X_f} f(X)X^{-\alpha_X} g(X/X_c)dX}^{\equiv I_1} + \overbrace{\int_{X_f}^{X_c} f(X)X^{-\alpha_X} g(X/X_c)dX}^{\equiv I_2} + \overbrace{\int_{X_c}^{\infty} f(X)X^{-\alpha_X} g(X/X_c)dX}^{\equiv I_3} \right) \tag{S2}$$

therefore $A_X = 1/(I_1 + I_2 + I_3)$ and

$$\lim_{N\to\infty} A_X = \frac{1}{\lim_{N\to\infty}(I_1 + I_2 + I_3)} \tag{S3}$$

In $I_1$ and $I_2$, we can approximate $g(X/X_c) \approx 1$ since $X < X_c$ in those integrals. In $I_2$ and $I_3$, $f(X) = 1$ by definition. Furthermore, assuming that $f(X)$ is independent of $N$, $I_1$ is also $N$-independent, and we therefore focus on $I_2 + I_3$,

$$I_2 + I_3 = \int_{X_f}^{X_c} X^{-\alpha_X} dX + \int_{X_c}^{\infty} X^{-\alpha_X} g(X/X_c)dX \tag{S4}$$

Using the variable $u \equiv X/X_c$ in the second integral, the expression becomes

$$I_2 + I_3 = \int_{X_f}^{X_c} X^{-\alpha_X} dX + X_c^{1-\alpha_X} \overbrace{\int_1^\infty u^{-\alpha_X} g(u)du}^{\equiv I_{U0}} \tag{S5}$$

Since $\alpha_X > 0$ and $g(u)$ tends to zero when $u \to \infty$ by definition, the integral $I_{U0}$ converges and is therefore just a constant, independent of $N$. To compute the left integral, we have two consider two cases: $\alpha_X \neq 1$ and $\alpha_X = 1$. If $\alpha_X \neq 1$, Eq. (S5) gives, after simplifying,

$$I_2 + I_3 = X_c^{1-\alpha_X} \cdot \left( \frac{1}{1-\alpha_X} + I_{U0} \right) + \frac{X_f^{1-\alpha_X}}{\alpha_X - 1} \text{ , for } \alpha_X \neq 1 \tag{S6}$$

The only $N$ dependence in Eq. (S6) comes from the term $X_c^{1-\alpha_X}$. Notice that, if $\alpha_X > 1$, $X_c^{1-\alpha_X}$ tends to zero in the limit $N \to \infty$ and Eq. (S6) tends to a constant, while, if $\alpha_X < 1$, $X_c^{1-\alpha_X}$ and therefore Eq. (S6) instead diverge to $+\infty$. If $\alpha_X = 1$ however, Eq. (S5) gives

$$I_2 + I_3 = \ln X_c - \ln X_f + I_{U0} \propto \ln X_c \propto \ln N \text{ , for } \alpha_X = 1 \tag{S7}$$

Since $\lim_{N\to\infty}(I_2+I_3)$ either tends to a constant or diverges to $+\infty$, we have $\lim_{N\to\infty}(I_1+I_2+I_3) \propto \lim_{N\to\infty}(I_2+I_3)$. Therefore, joining all cases, we have

$$\lim_{N\to\infty}(I_1+I_2+I_3) \propto \begin{cases} \text{constant} & \text{for } \alpha_X > 1 \\ \ln N & \text{for } \alpha_X = 1 \\ N^{\beta_X\cdot(1-\alpha_X)} & \text{for } \alpha_X < 1 \end{cases} \tag{S8}$$

Using this result in (S3), we obtain

$$\boxed{\lim_{N\to\infty} A_X \propto \begin{cases} \text{constant} & \text{for } \alpha_X > 1 \\ 1/\ln N & \text{for } \alpha_X = 1 \\ N^{-\beta_X\cdot(1-\alpha_X)} & \text{for } \alpha_X < 1 \end{cases}} \tag{S9}$$

### S2.2. Large $N$ limit of $\langle X\rangle$

The average $\langle X\rangle = \int_1^\infty XP(X)dX$ is given by, again defining $X_f$ such that $f(X) = 1$ for $X > X_f$ and separating the integral into three parts,

$$\langle X\rangle = A_X \cdot \left( \overbrace{\int_1^{X_f} f(X)X^{1-\alpha_X}dX}^{\equiv I_4} + \overbrace{\int_{X_f}^{X_c} X^{1-\alpha_X}dX}^{\equiv I_5} + \overbrace{\int_{X_c}^{\infty} X^{1-\alpha_X}g(X/X_c)dX}^{\equiv I_6} \right) \tag{S10}$$

where we used $g(X/X_c) \approx 1$ in $I_4$ and $I_5$ since $X < X_c$ in those integrals, and $f(X) = 1$ in $I_5$ and $I_6$ by definition. To estimate the scaling of $\lim_{N\to\infty}\langle X\rangle = \lim_{N\to\infty}(A_X)\lim_{N\to\infty}(I_4+I_5+I_6)$, we have first to understand the behaviour of $\lim_{N\to\infty}(I_4+I_5+I_6)$. Notice that $I_4+I_5+I_6$ is just $I_1+I_2+I_3$ but with $\alpha_X$ replaced by $\alpha_X - 1$. A particular point for caution is that the integral analogous to $I_{U0}$, given by $I_{U1} \equiv \int_1^\infty u^{1-\alpha_X}g(u)du$, has the term $u^{1-\alpha_X}$ that diverges when $u \to \infty$ if $\alpha_X < 1$. However, the rapid decay of $g(u)$ ensures that $I_{U1}$ also converges to a constant even for $\alpha_X < 1$. Thus, using Eq. (S8),

$$\lim_{N\to\infty}(I_4+I_5+I_6) \propto \begin{cases} \text{constant} & \text{for } \alpha_X > 2 \\ \ln N & \text{for } \alpha_X = 2 \\ N^{\beta_X\cdot(2-\alpha_X)} & \text{for } \alpha_X < 2 \end{cases} \tag{S11}$$

Finally, using Eq. (S11) and (S9), we can estimate the scaling of $\lim_{N\to\infty}\langle X\rangle \propto \lim_{N\to\infty}(A_X)\lim_{N\to\infty}(I_4+I_5+I_6)$ for all the possible cases depending on $\alpha_X$,

$$\boxed{\lim_{N\to\infty}\langle X\rangle \propto \begin{cases} \text{constant} & \text{for } \alpha_X > 2 \\ \ln N & \text{for } \alpha_X = 2 \\ N^{\beta_X\cdot(2-\alpha_X)} & \text{for } 1 < \alpha_X < 2 \\ N^{\beta_X}/\ln N & \text{for } \alpha_X = 1 \\ N^{\beta_X} & \text{for } \alpha_X < 1 \end{cases}} \tag{S12}$$

recalling that $\alpha_X$ is the power-law exponent of the avalanche size or duration distribution and $\beta_X$ is the exponent of the scaling of the cut-off $X_c$ with $N$.

## S3. QUIET TIMES FOR THE MANNA MODEL

We compute the distribution of quiet times for the Manna model. The rule is that at each step one grain is added to a random site $i$ with height $h_i$ until an avalanche is triggered. In the steady-state a stable configuration will be composed by $n$ occupied sites and $N-n$ empty sites. An avalanche is triggered if the new grain falls into an occupied site (a site with $h_i = 1$), otherwise the number of occupied sites is increased to $n+1$. We want to know the probability that an occupied site is picked for the first time after $k$ attempts.

This problem is equivalent to the following one: We are given $N$ balls in a box, out of which $n$ are white and $N-n$ are black. At each step, one ball is randomly picked. If the ball is black, it is replaced with a white ball. We are interested in finding the probability that the first white ball is picked exactly after $k$ steps.

### S3.1. Solution

Initially, there are $n$ white balls and $N-n$ black balls in the box. In order to pick the first white ball at the $k$-th step, it is necessary that black balls are picked in each of the first $k-1$ steps. The probability of picking a black ball at step $i$ (for $i = 1, 2, \ldots, k-1$) is given by

$$P(\text{pick black at step } i) = \frac{N-n-(i-1)}{N} \tag{S13}$$

On the $k$-th step, the probability of picking a white ball is

$$P(\text{pick white at step } k) = \frac{n+k-1}{N} \tag{S14}$$

The probability of picking the first white ball at step $k$ is the product of the probabilities of picking black balls for the first $k-1$ steps, followed by picking a white ball on the $k$-th step

$$P(\text{first white at step } k) = \left(\prod_{i=1}^{k-1} \frac{N-n-(i-1)}{N}\right) \frac{n+k-1}{N} \tag{S15}$$

Expanding the product, this gives

$$\boxed{P(\text{first white at step } k) = \frac{(N-n)\cdot(N-n-1)\cdots(N-n-(k-2))\cdot(n+k-1)}{N^k}} \tag{S16}$$

### S3.2. Limit for large $N$ with $n/N = p$

Now, we consider the limit as $N \to \infty$ while maintaining $n/N = p$, where $p$ is the fraction of white balls. In the Manna model $p$ is the fraction of occupied sites in the steady state, that is known to be constant. Using $n = pN$, the probability (S16) becomes

$$P(\text{first occupied site at step } k) = \frac{(N\cdot(1-p))\cdot(N\cdot(1-p)-1)\cdots(N\cdot(1-p)-(k-2))\cdot(pN+k-1)}{N^k} \tag{S17}$$

For large $N$, we approximate each term

$$N\cdot(1-p) - i \approx N\cdot(1-p) \text{ , for } i \ll N, \tag{S18}$$

and

$$pN + k - 1 \approx pN \tag{S19}$$

Therefore, the probability (S17) simplifies to

$$P(\text{first occupied site at step } k) \approx \frac{(N\cdot(1-p))^{k-1} pN}{N^k} \tag{S20}$$

Canceling $N^{k-1}$ from both the numerator and denominator, we get the geometric distribution

$$\boxed{P(\text{first occupied site at step } k) \approx p \cdot (1-p)^{k-1} \text{ , for large } N} \tag{S21}$$

Therefore, the average number of steps $\langle k \rangle$ before picking an occupied site is given by $1/p$ for large $N$. The quiet time $\tau$ in the Manna model corresponds to $k-1$, so the average $\langle \tau \rangle$ is given by

$$\boxed{\langle \tau \rangle \approx \frac{1}{p} - 1, \text{ for large } N} \tag{S22}$$

[1] Alessandro Chessa, Alessandro Vespignani, and Stefano Zapperi. Critical exponents in stochastic sandpile models. *Computer Physics Communications*, 121–122:299–302, September 1999.
